# Supplementary material for: MSTC*:Multi-robot Coverage Path Planning under Physical Constraints
Source: arXiv:2108.04632 source file (2021-08-10)
Supplement: Supplementary file 1 [file appendix.tex]

\section*{APPENDIX}
